# Supplementary material for: Human-AI Guidelines in Practice: Leaky Abstractions as an Enabler in Collaborative Software Teams
Source: arXiv:2207.01749 source file (2022-07-04)
Supplement: Supplementary file 1 [file appendix.tex]

\appendix

\section{Semi-Structured Interview Questions} \label{interview-questions}

\begin{enumerate}
    \item \revisions{What is your role at your company?}
    \item \revisions{How big is your team size? }
    \item \revisions{What is the organization structure like in your team? What are the roles of different people in the team? designer? front end developer? backend? AI?}  
    \item \revisions{Can we choose one AI-based application you helped design/develop (that you can speak about) ? Can you describe the application and the specific AI features it implements?}
    \item \revisions{Can you walk me through the process of creating the AI-based application? When walking us through, can you describe in detail the different roles that were involved?}
        \begin{itemize}[label=\textcolor{blue}{\textbullet}]
            \item \revisions{(designer) Can you talk us through the design process you took to design the AI features? Please be specific about how you discovered user needs, how you developed the idea for the feature, and how you designed the interaction around it.}
            \item \revisions{(designer/ux researcher) When you build this application, how do you go about telling users that these things are automated for you? How do you build their expectation using a design aspect?}
            \item \revisions{(engineer/scientist) Can you tell me about how you got the requirements for this feature? Did you have the data, or did you or others need to collect new data? Were there any challenges obtaining the data?}
            \item \revisions{(engineer/scientist) How much say do you have on the overall product’s user experience in the process?}
        \end{itemize}
    
     \item \revisions{How did you collaborate with [role name]?}
        \begin{itemize}[label=\textcolor{blue}{\textbullet}]
            \item \revisions{(designer) How did you collaborate with the engineering team to design and develop this feature?}
            \item \revisions{(engineer) How did you collaborate with UX designers when developing this feature? Can you explain the interactions and what inputs or feedback you received?}
        \end{itemize}
        
    \item \revisions{Were there any conflicts with AI engineers/designers/different roles? How did you resolve it?}
    
     \item \revisions{How did you evaluate the feature?}
        \begin{itemize}[label=\textcolor{blue}{\textbullet}]
            \item \revisions{(designer) Did you evaluate this feature with users? Who evaluates the AI side of this?}
            \item \revisions{(engineer) How did you evaluate this feature/ AI model?}
        \end{itemize}
     
    \item \revisions{Did you refer to any design guidelines when creating this feature? What tools did you use? Are those tools in house?}
    \item \revisions{Are there any tools that you wish you had?}

    \item \revisions{What are some kinds of prototypes that are involved in creating the application? Can you walk me through the process of making those prototypes? Can you tell me about the collaborative/communicative aspects of prototypes?}

    \item \revisions{What do you think are the main differences between developing AI driven applications, and those that don’t involve AI? What are the similarities?}

    \item \revisions{What do you think about the recent design guidelines for human AI applications being released by companies? }

    \item \revisions{What were the challenges you faced in collaborations with other roles? What do you think would be an ideal workflow for collaboratively building AI-based applications? }
    \begin{itemize}[label=\textcolor{blue}{\textbullet}]
        \item \revisions{(designer) As a designer, how much about the AI do you think you'll need to know in order to provide for a good user experience?}
    \end{itemize}
\end{enumerate}

\section{Coding Scheme} \label{codes}
