# Supplementary material for: Human-AI Guidelines in Practice: Leaky Abstractions as an Enabler in Collaborative Software Teams
Source: arXiv:2207.01749 source file (2022-07-04)
Supplement: Supplementary file 2 [file 08_appendixA.tex]

\section{Questions for Semi-Structured Interviews}
