# Supplementary material for: Human-AI Guidelines in Practice: Leaky Abstractions as an Enabler in Collaborative Software Teams
Source: arXiv:2207.01749 source file (2022-07-04)
Supplement: Supplementary file 3 [file 09_appendixB.tex]

\section{Codebook}
